# Supplementary material for: P3P: Pseudo-3D Pre-training for Scaling 3D Voxel-based Masked Autoencoders
Source: arXiv:2408.10007 source file (2025-05-21)
Supplement: Supplementary file 1 [file appendix.tex]

\clearpage
\section{Appendix}

\subsection{t-SNE visualization}

\begin{figure}[t]
    \centering
    \includegraphics[width=0.48\textwidth]{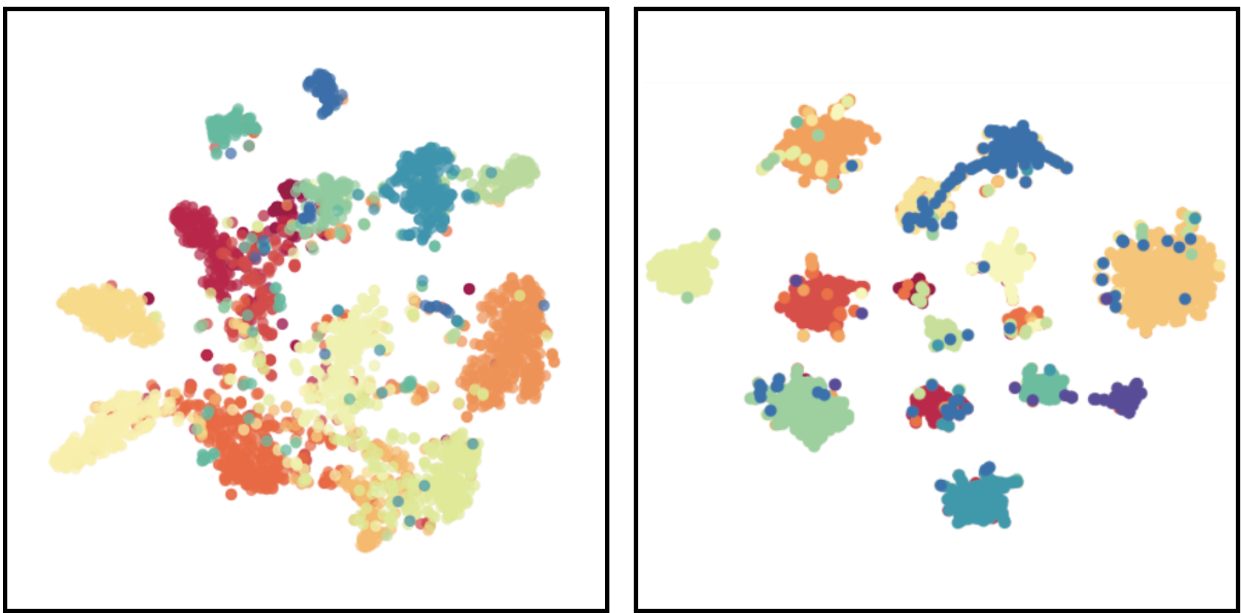}
    \caption{Visualization of feature distributions. We show the t-SNE visualization of feature vectors after fine-tuning on the ScanObjectNN PB\_T50\_RS classification dataset. We make a comparison between Point-BERT(left) and ours(right).}
    \label{fig:tsne}
\end{figure}

\paragraph{Visualization.}
We visualize the pseudo-3D data in Fig.~\ref{fig:demo}.
Various objects from indoor to outdoor, from small to big, from colorful to to plain, are introduced to 3D pre-training corpora.

\begin{figure}[h]
    \centering
    \includegraphics[width=0.45\textwidth]{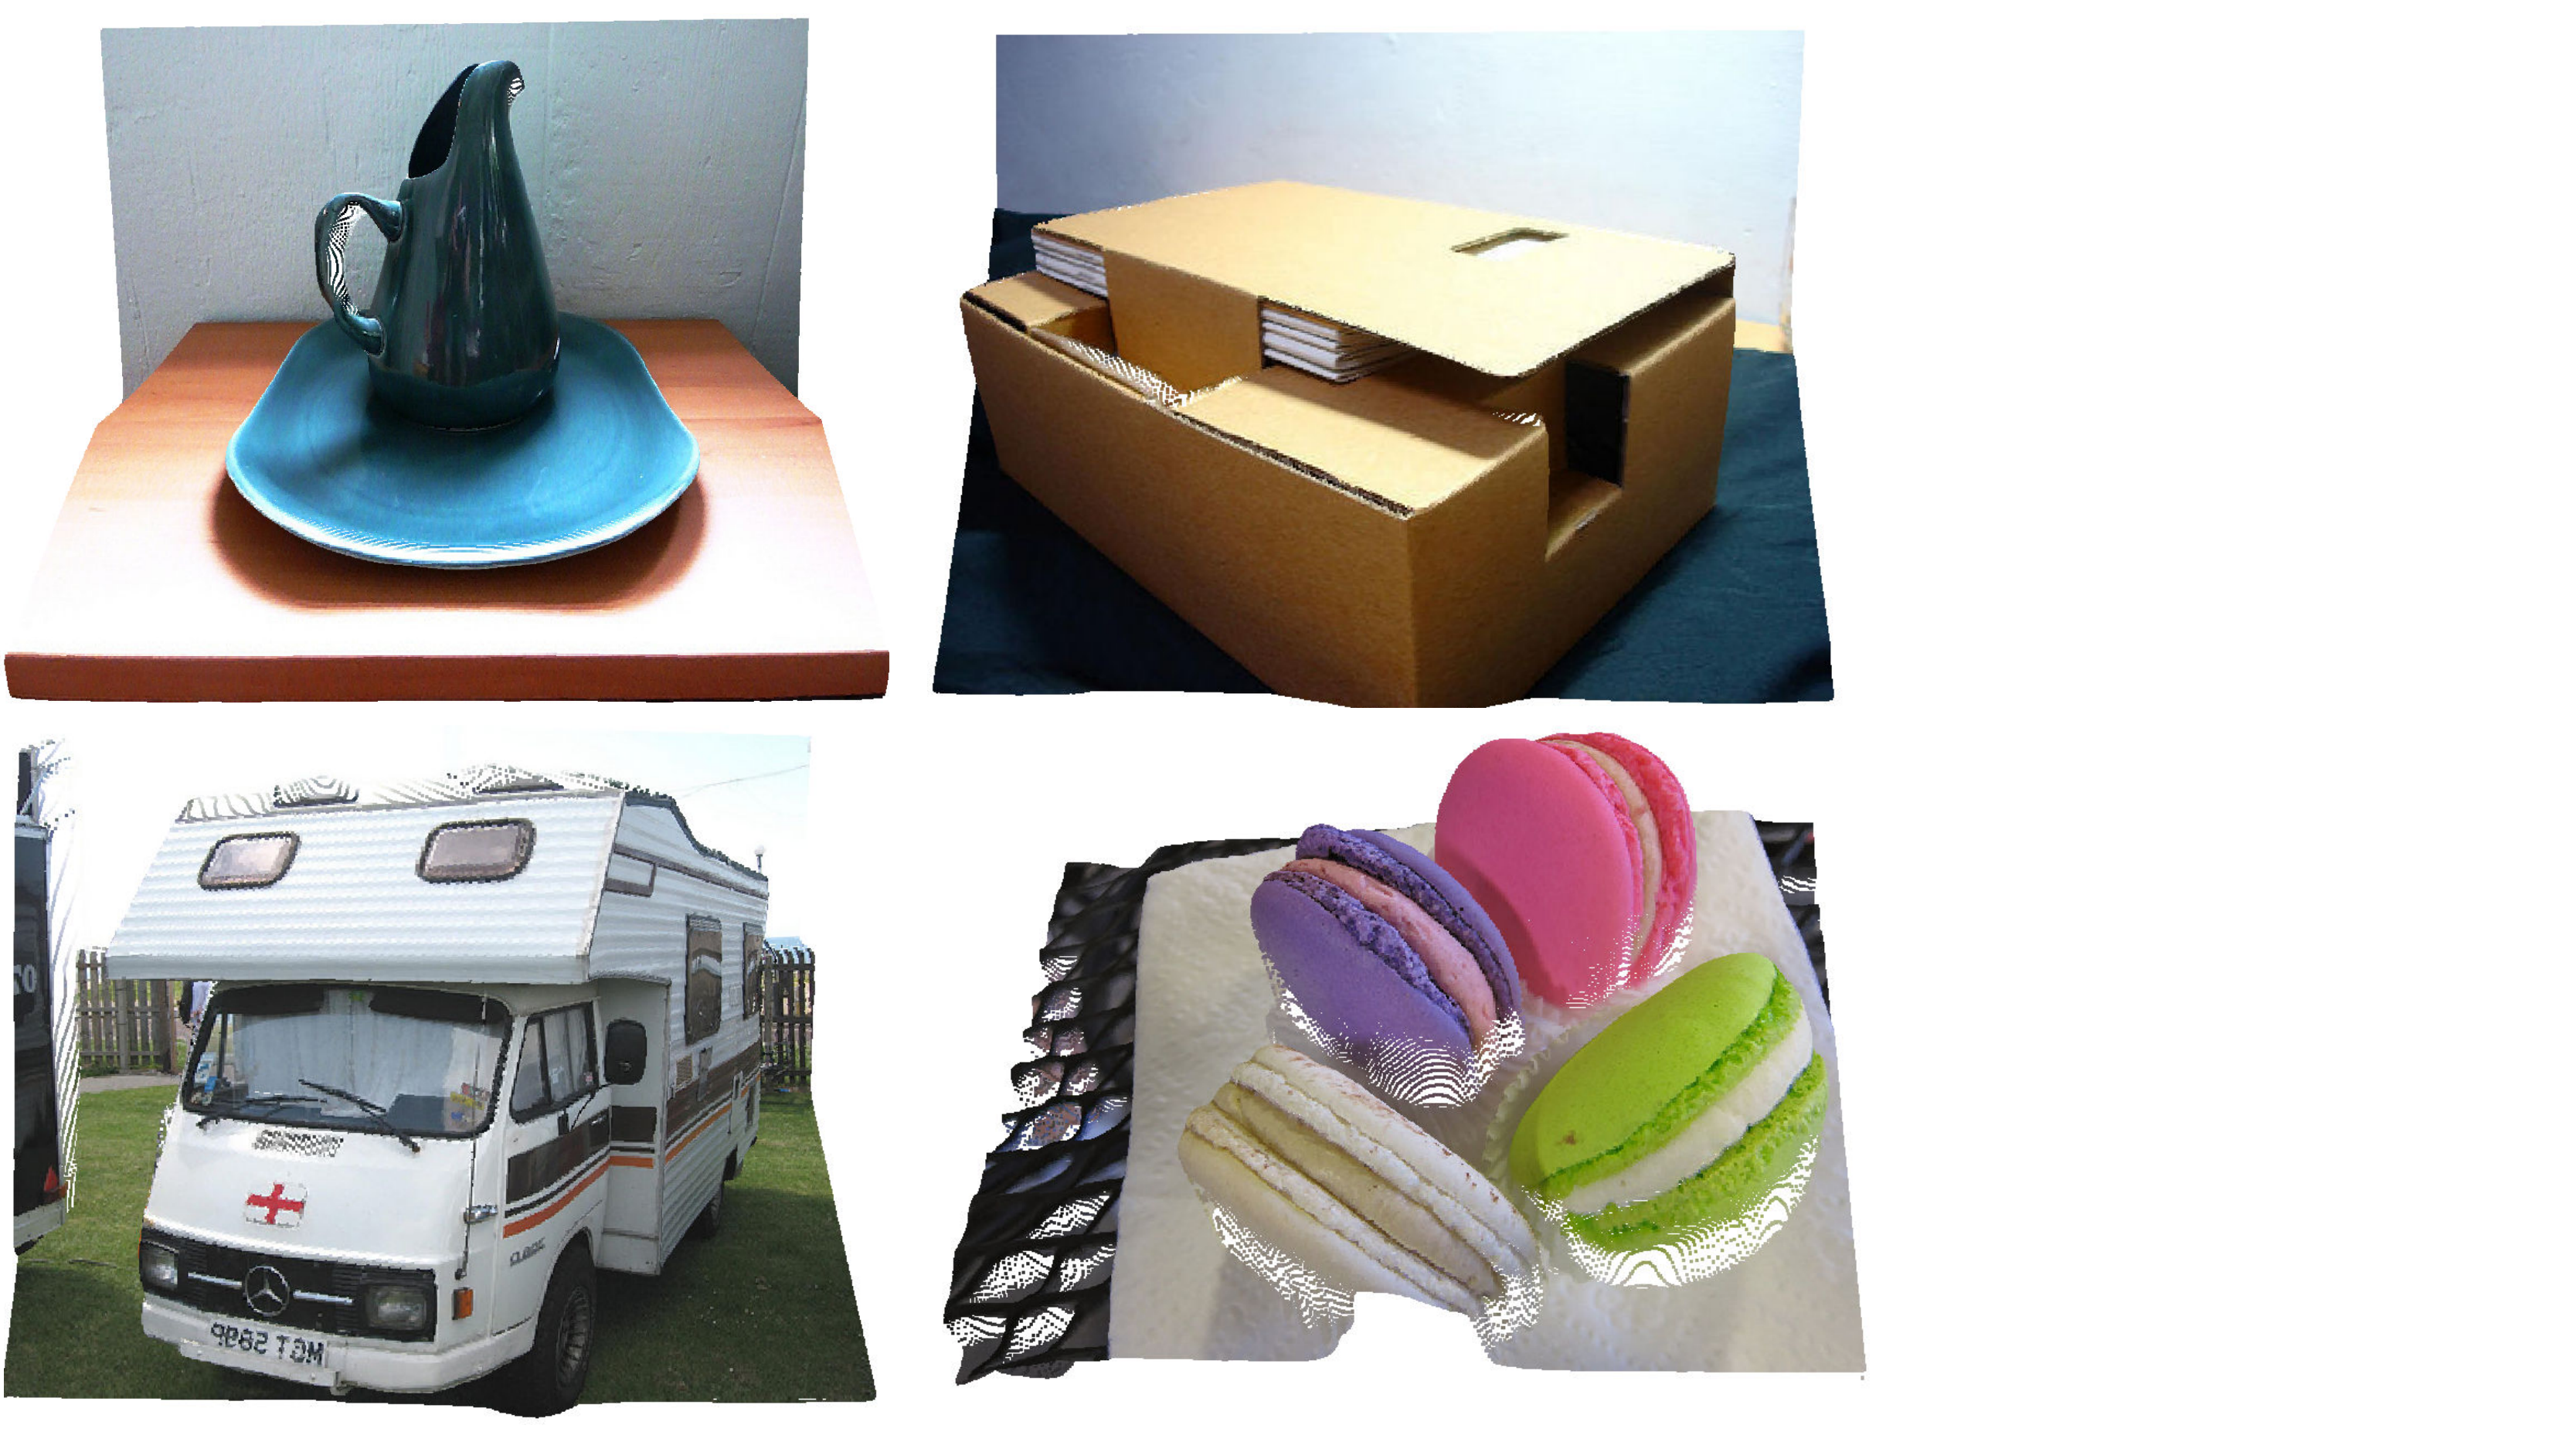}
    \caption{Pseudo-3D data lifted from ImageNet. Abundant geometry and color information are introduced to 3D pre-training corpora by depth estimation.\label{fig:demo}}
\end{figure}

\subsection{Code Implementation Details}
We promise the full code repository and the corresponding instructions for reproducing the pre-training and fine-tuning results will be published before the paper's publication.
We show our core Python code and explain it in this section.

\paragraph{Create pseudo-3D data.}
We show our core Python code for creating pseudo-3D data in Fig.~\ref{fig:createdata}.
Given images and the predicted depth from Depth Anything Large models, we first normalize the colors and the depth.
Then we produce the discrete $x-axis$ and $y-axis$, and normalize them.
Finally, we stack the 3 axes and concatenate with colors to get the pseudo-3D point cloud.
All features of the point cloud are normalized to a canonical space.

\paragraph{Token embedding.}
We show our core Python code for token embedding in Fig.~\ref{fig:code}.
Line $64$ shows the weights definition of our proposed Sparse Weight Indexing. 
Line $69$ shows how the embedding works.
First, the corresponding weights are indexed by $coords\_rela\_query$, which is achieved by Eq.\ref{eq:indexing} in our Approach section.
Note that the indexes range from $0$ to $16^3-1$ and repeat many times such that the weights are shared across different 3D patches.
Function $scatter$ is imported from the $torch\_scatter$ library, which can perform scatter operations across different batches/patches with different lengths.
And the $reduce$ argument is set to $mean$, which is equal to the Eq.~\ref{eq:embedding} in our Approach section.
It is worth noting that, our token embedding is mathematically equal to the token embedding of MAE and ViT.
The difference is that ours performs on sparse data while theirs performs on dense data.

\paragraph{Positional embedding.}
We show our core Python code for positional embedding in Fig.~\ref{fig:code}.
Line $52$ to $56$ shows the positional embedding of our encoder and line $59$ to $63$ shows the positional embedding of our decoder, following Point-MAE.

\paragraph{Reconstruction target.}
We show our core Python code for reconstruction targets in Fig.~\ref{fig:code}.
The two $124$ lines show the 2D reconstruction target same as MAE and the 3D reconstruction target we make a comparison.
We predict the 2D space $patch\_size^2$ of a 2D patch and predict the 3D space $patch\_size^3$ of a 3D patch.
In our Experiment section, we make a thorough comparison between the two reconstruction targets and prove the 2D reconstruction target is more device-friendly than the 3D, meanwhile maintaining roughly the same downstream classification accuracy.

\begin{figure}[t]
    \centering
    \includegraphics[width=0.47\textwidth]{figures/createdata.png}
    \caption{Core Python code for our pseudo-3D data creation.\label{fig:createdata}}
\end{figure}

\begin{figure*}[t]
    \centering
    \includegraphics[width=\textwidth]{figures/code appendix.pdf}
    \caption{Core Python code for our embedding and reconstruction targets.\label{fig:code}}
\end{figure*}

\subsection{Visualization of More Pseudo-3D Data}
We visualize the pseudo-3D data in Fig.~\ref{fig:demo2}.
Various objects from indoor to outdoor, from small to big, from colorful to to plain, are introduced to 3D pre-training corpora.

\subsection{Visualization of the Reconstructed Target}
MAE formulates a generative pre-training paradigm. In the original MAE paper, they demonstrated some reconstructed samples.
We take screenshots from their paper in Fig.~\ref{fig:demo4} to compare with our results.
We also show our reconstructed samples in Fig.~\ref{fig:demo3}.
We observe that our reconstructed results share features similar to those of MAE: At a high masking ratio (ours $60\%$, MAE $80\%$), the transformer decoder can reconstruct the roughly correct color but blurred texture.

\begin{figure*}[t]
    \centering
    \includegraphics[width=\textwidth]{figures/demo2.pdf}
    \caption{Pseudo-3D data lifted from ImageNet. Abundant geometry and color information are introduced to 3D pre-training corpora by depth estimation.\label{fig:demo2}}
\end{figure*}

\begin{figure*}[t]
    \centering
    \includegraphics[width=\textwidth]{figures/reconstruct target.pdf}
    \caption{The left column shows the masked 3D patches (ground truth) of pseudo-3D samples. The middle column shows the reconstructed 3D patches generated by our transformer decoder. The right column shows the original full pseudo-3D samples. \label{fig:demo3}}
\end{figure*}

\begin{figure*}[t]
    \centering
    \includegraphics[width=\textwidth]{figures/mae_reconstructed.pdf}
    \caption{This is a screenshot taken from the MAE paper. The left column shows the masked images fed to MAE's transformer decoder. The middle column shows the reconstructed images generated by MAE's transformer decoder. The right column shows the original images. \label{fig:demo4}}
\end{figure*}
